# Supplementary material for: NOVA: A visual interface for assessing polarizing media coverage
Source: arXiv:2403.00334 source file (2024-03-01)
Supplement: Supplementary file 1 [file appendix.tex]

% \section{Modals}
\noindent Below are the modals that automatically pops up when the user enter each stage. The modals explains the context of the page and the task that is expected to be done. These modals supports sensemaking and keeps user engaged throughout the self-assessment of personal belief with NOVA.
\begin{figure}[h]
    \centering
    \includegraphics[keepaspectratio, width=\columnwidth]{figures/Modals/overview_modal.png}
    \caption{Modal of the Topic Selection Stage explaining the purpose of NOVA and the displayed dataset. At the end, the modal invites users to explore the topics in the first stage.}
    \label{fig: second-overview-modal}
\end{figure}

\begin{figure}[h]
    \centering
    \includegraphics[keepaspectratio, width=\columnwidth]{figures/Modals/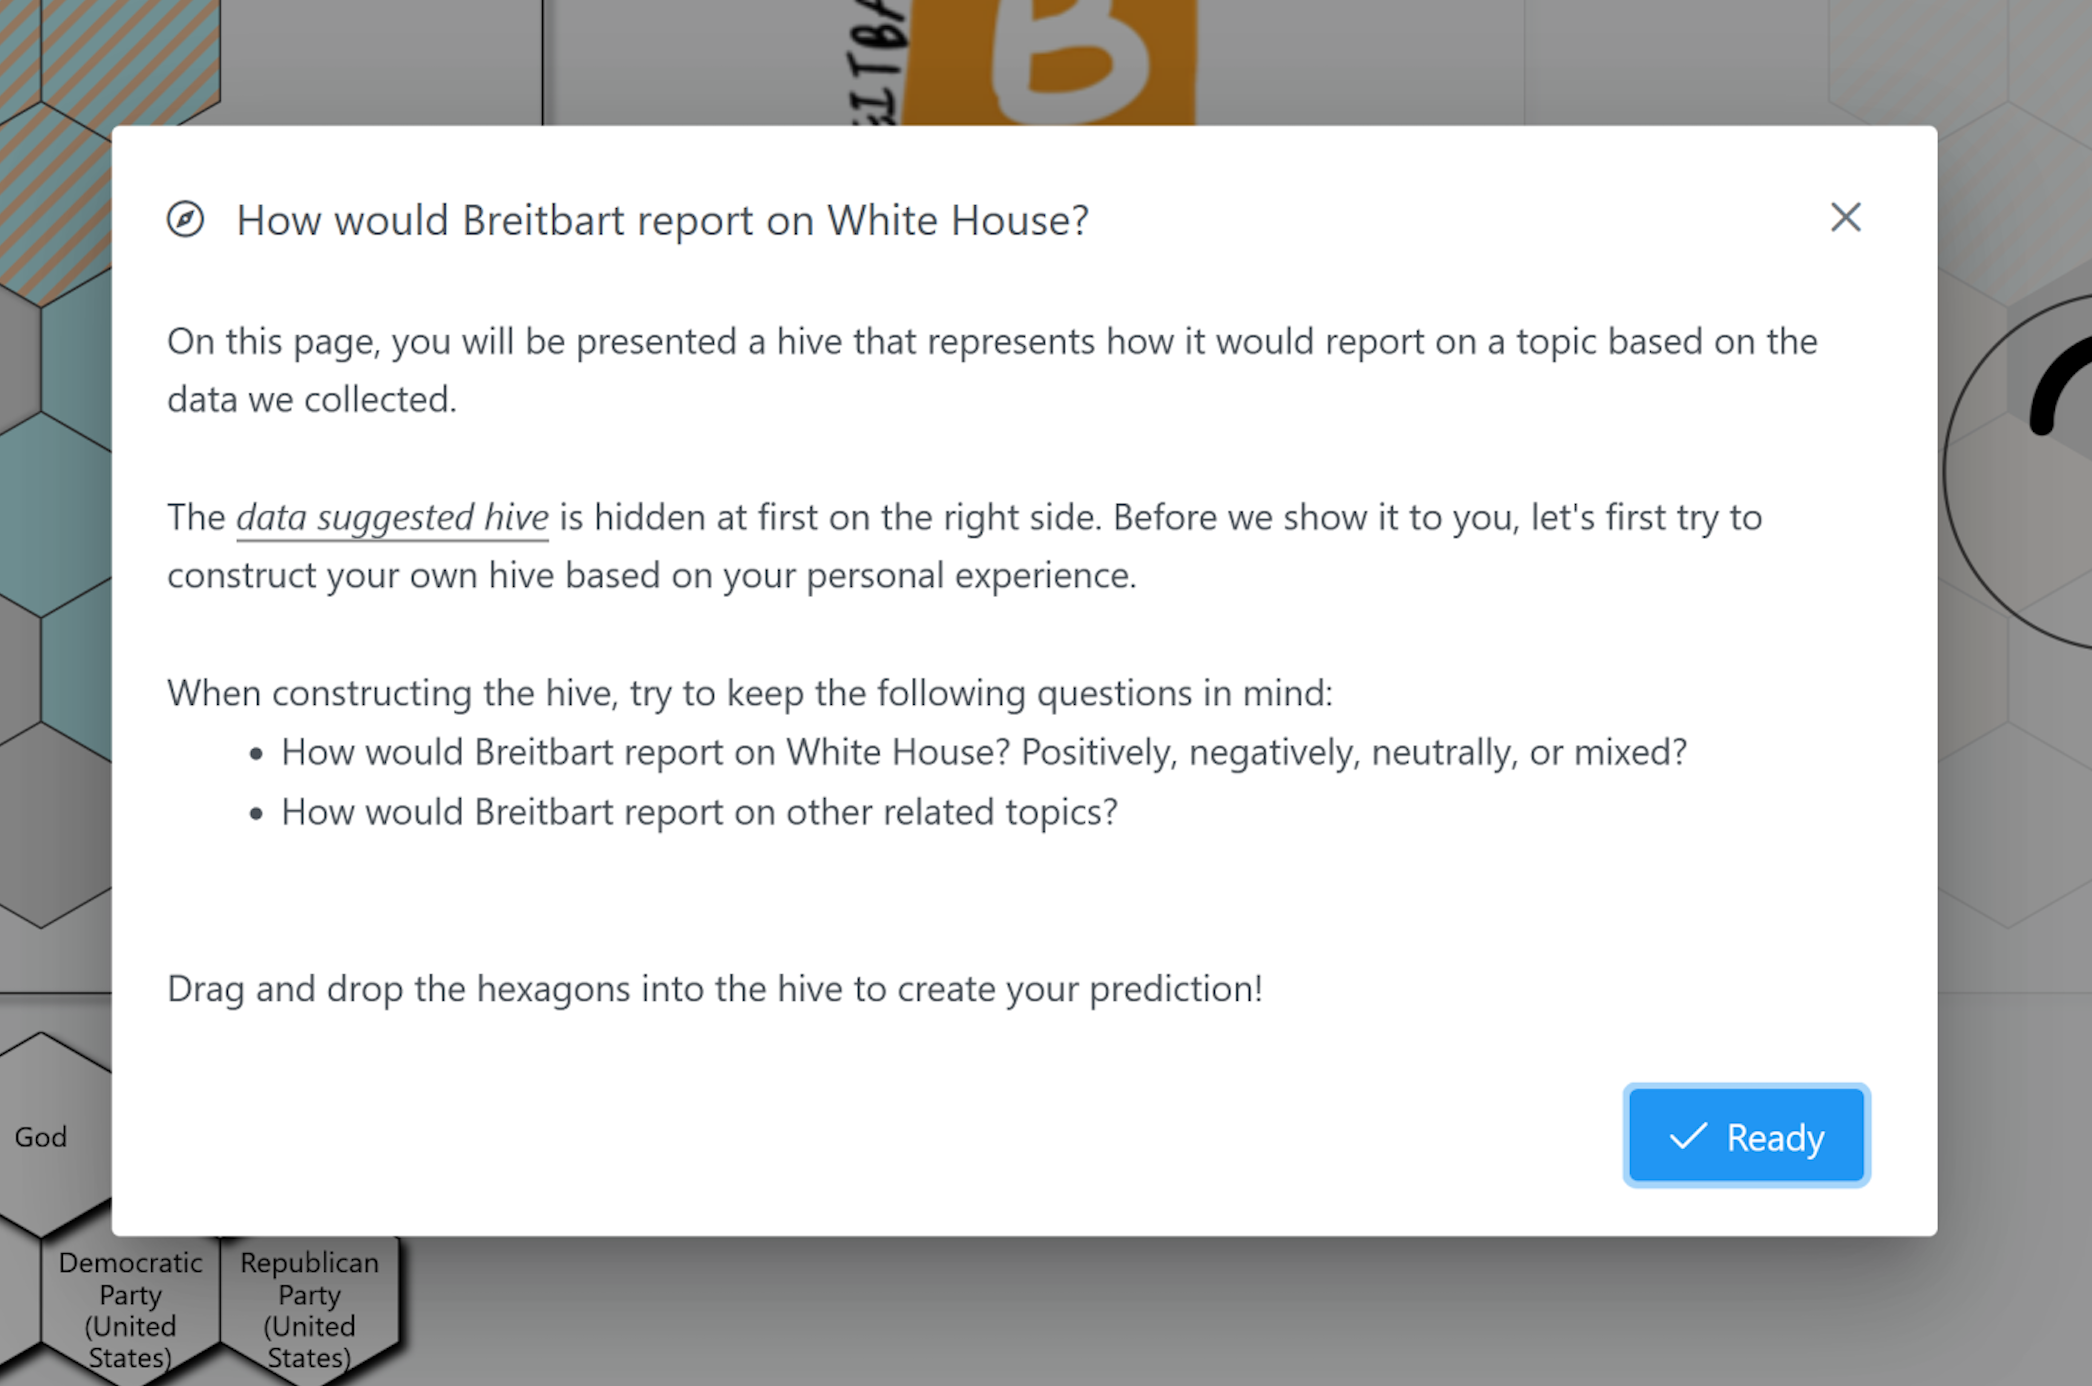}
    \caption{Modal the Belief Elicitation stage explaining the topic hives that compares personal belief and the data. It explains the interactions and prompts the user with two questions before entering the stage.}
    \label{fig: second-overview-modal}
\end{figure}

\begin{figure}[h]
    \centering
    \includegraphics[keepaspectratio, width=\columnwidth]{figures/Modals/article_modal.png}
    \caption{Modal of the Article Review Stage explaining the expected task to be done with the stage: find evidence to support or disprove personal belief.}
    \label{fig: second-overview-modal}
\end{figure}
